# Supplementary material for: Mass transport computations via correlation splitting and a law of total diffusion
Source: arXiv:2112.01978 source file (2021-12-03)
Supplement: Supplementary file 1 [file SM.pdf]

# I. BRIDGING LAW BETWEEN THE LAWS OF TOTAL DIFFUSION AND VARIANCE FOR EQUILIBRIUM DISPLACEMENTS: DERIVATION FROM THE LAW OF TOTAL COVARIANCE

At equilibrium, any mean displacement vector is zero whatever $\ell$: $\mathbb{E}[\mathbf{r}_{0\to\ell}] = 0$. Hence, the mean squared displacement tensor corresponds to the variance-covariance matrix $\mathbb{V}[\mathbf{r}_{0\to\ell}]$ with $\mathbb{V}[\mathbf{x}] = \mathbb{C}\mathrm{ov}[\mathbf{x},\mathbf{x}]$ and where $\mathbb{C}\mathrm{ov}[\mathbf{x},\mathbf{y}] = \mathbb{E}[\mathbf{x}\otimes\mathbf{y}] - \mathbb{E}[\mathbf{x}]\otimes\mathbb{E}[\mathbf{y}]$ denotes the covariance matrix of $\mathbf{x}$ and $\mathbf{y}$ vectors. For convenience, we hereafter consider the variance $\mathbb{V}[\mathbf{r}_{0\to\ell}]$ instead of the diffusion matrix $\mathbb{D}_\ell[\mathbf{r}_{0\to 1}]$. Reverting to the diffusion matrix is straightforward from relationship:

$$\mathbb{V}[\mathbf{r}_{0\to\ell}] = 2\ell\mathbb{D}_\ell[\mathbf{r}_{0\to 1}]\,\mathbb{E}[t_1 - t_0]. \tag{S1}$$

The variance of the $\ell$ displacements can be decomposed with the help of the covariance of the individual displacements:

$$\mathbb{V}[\mathbf{r}_{0\to\ell}] = \sum_{k=0}^{\ell-1}\sum_{l=0}^{\ell-1}\mathbb{C}\mathrm{ov}[\mathbf{r}_{k\to k+1},\mathbf{r}_{l\to l+1}] \tag{S2}$$

Resorting to translational invariance, the double summation in (S2) simplifies into a single summation in (S3):

$$\mathbb{V}[\mathbf{r}_{0\to\ell}] = \sum_{k=1}^{\ell}\mathbb{V}[\mathbf{r}_{k\to k+1}] + 2(\ell-k)\mathbb{C}\mathrm{ov}[\mathbf{r}_{k\to k+1},\mathbf{r}_{0\to 1}]\,. \tag{S3}$$

We now implement a conditioning scheme in both the variance and covariance appearing in the summation of equation (S3). One must distinguish the first term entailing a variance ($k=0$) from the subsequent autocovariance terms ($k>0$). We first apply the law of total variance on the first term, with conditioning on $\chi_1$, which yields

$$\mathbb{V}[\mathbf{r}_{k\to k+1}] = \mathbb{E}[\mathbb{V}[\mathbf{r}_{k\to k+1}|\chi_k]] + \mathbb{V}[\mathbb{E}[\mathbf{r}_{k\to k+1}|\chi_k]]\,. \tag{S4}$$

Next, the law of total covariance on the extra terms, with conditioning on $\chi_1,\cdots,\chi_k$ over $\chi_0$ and $\chi_{k+1}$, yields ($k>0$)

$$\mathbb{C}\mathrm{ov}[\mathbf{r}_{k\to k+1},\mathbf{r}_{0\to 1}] = \mathbb{E}[\mathbb{C}\mathrm{ov}[\mathbf{r}_{k\to k+1},\mathbf{r}_{0\to 1}|\chi_1,\cdots,\chi_k]] + \mathbb{C}\mathrm{ov}[\mathbb{E}[\mathbf{r}_{k\to k+1}|\chi_k],\mathbb{E}[\mathbf{r}_{0\to 1}|\chi_1]]\,. \tag{S5}$$

When conditioning is done on $\chi_1,\cdots,\chi_k$, then we have $\mathbb{C}\mathrm{ov}[\mathbf{r}_{k\to k+1},\mathbf{r}_{0\to 1}|\chi_1,\cdots,\chi_k] = 0$, since $\chi_0$ and $\chi_{k+1}$ are uncorrelated. Hence, the expected conditional covariance, i.e. the first term of the right-hand side of (S5), cancels. We are left with

$$\mathbb{C}\mathrm{ov}[\mathbf{r}_{k\to k+1},\mathbf{r}_{0\to 1}] = -\mathbb{C}\mathrm{ov}[\mathbb{E}[\mathbf{r}_{k\to k+1}|\chi_k],\mathbb{E}[\mathbf{r}_{1\to 2}|\chi_1]]\,, \tag{S6}$$

where we resorted to the reversibility and translation property of the Markov process and replaced $\mathbb{E}[\mathbf{r}_{0\to 1}|\chi_1]$ by $-\mathbb{E}[\mathbf{r}_{1\to 2}|\chi_1]$ in the last equation.

The summed covariance in (S3) can be expressed using the laws of total variance (S4) and covariance (S6), which leads to:

$$\begin{aligned}
\mathbb{V}[\mathbf{r}_{0\to\ell}] &= \sum_{k=1}^{\ell}\left\{\mathbb{E}[\mathbb{V}[\mathbf{r}_{k\to k+1}|\chi_k]] + \mathbb{V}[\mathbb{E}[\mathbf{r}_{1\to 2}|\chi_1]] - 2(\ell-k)\mathbb{C}\mathrm{ov}[\mathbb{E}[\mathbf{r}_{k\to k+1}|\chi_k],\mathbb{E}[\mathbf{r}_{1\to 2}|\chi_1]]\right\}\\
&= \ell\mathbb{E}[\mathbb{V}[\mathbf{r}_{1\to 2}|\chi_1]] + \mathbb{V}[\mathbb{E}[\mathbf{r}_{1\to 2}|\chi_1]] - \sum_{k=2}^{\ell}\left\{\mathbb{V}[\mathbb{E}[\mathbf{r}_{1\to 2}|\chi_1]] + 2(\ell-k)\mathbb{C}\mathrm{ov}[\mathbb{E}[\mathbf{r}_{k\to k+1}|\chi_k],\mathbb{E}[\mathbf{r}_{1\to 2}|\chi_1]]\right\}\\
&= \ell\mathbb{E}[\mathbb{V}[\mathbf{r}_{1\to 2}|\chi_1]] + \mathbb{V}[\mathbb{E}[\mathbf{r}_{1\to 2}|\chi_1]] - \mathbb{V}\left[\sum_{k=1}^{\ell-1}\mathbb{E}[\mathbf{r}_{k\to k+1}|\chi_k]\right]\,.
\end{aligned} \tag{S7}$$

At equilibrium, mean displacements are zero, and translational invariance holds, thus we have the simplification

$$\frac{1}{\ell}\mathbb{V}[\mathbf{r}_{0\to\ell}] = \mathbb{E}[\mathbb{V}[\mathbf{r}_{0\to 1}|\chi_0]] + \frac{1}{\ell}\left\{\mathbb{V}[\mathbb{E}[\mathbf{r}_{0\to 1}|\chi_0]] - \mathbb{V}\left[\sum_{k=1}^{\ell-1}\mathbb{E}[\mathbf{r}_{k\to k+1}|\chi_k]\right]\right\}\,. \tag{S8}$$

The relationship bridges between the law of total variance for $\ell = 1$ (Eq. 7 of article) and the law of total diffusion (Eq. 9 of article), obtained after dividing by $2\mathbb{E}[t_1 - t_0]$ for $\ell\to\infty$.

## II. CONVENTIONAL KMC SIMULATIONS WITH MODERATE DYNAMICAL TRAPPING

We have performed additional kMC simulations with moderate dynamical trapping to investigate the behavior of the conditioned estimator. We have set the frequencies $\nu_A$ to 1 and $\nu_B$ to 5. We have repeated the kPS simulations presented in the core article using the conventional kMC algorithm with moderate dynamical trapping. Diffusion coefficients are estimated using $10^6$ trajectories of $\ell_{\max} = 10^4$ kMC steps. Other simulation setups are identical (lattice size and periodic boundary conditions). The measured diffusion coefficients are reported in Fig. S1. We also report the convergence properties of the diffusion coefficients as a function of the path length $\ell$ in Fig. S2 for $C_B = 39\%$ and Fig. S3 for $C_B = 61\%$. The observed trends for the simulation speed-ups are similar to the case of extreme dynamical trapping. The accuracy is overall much improved by conditioning, except for isolated $B$-clusters at low $B$-composition whose motion remains limited. A difference concerns the visible effect of increasing $B$-concentation on $A$-diffusivity that moderately decreases, while $A$-diffusivity still increases monotonously but much more smoothly. In contrast to kPS simulations, standard errors of the conditioned estimates also comes from the extra-correlated contribution to diffusion. We also note that the conditioned estimator is less efficient than the standard one whenever the control variate is lower than half. This situation occurs at low $B$ compositions for which clusters are isolated and immobile for long periods of time prior to being visited by the vacancy again. This specific regime of intermittent trapping is not captured by the intra-correlated part and explain the relatively lower performance of the conditioned estimator.

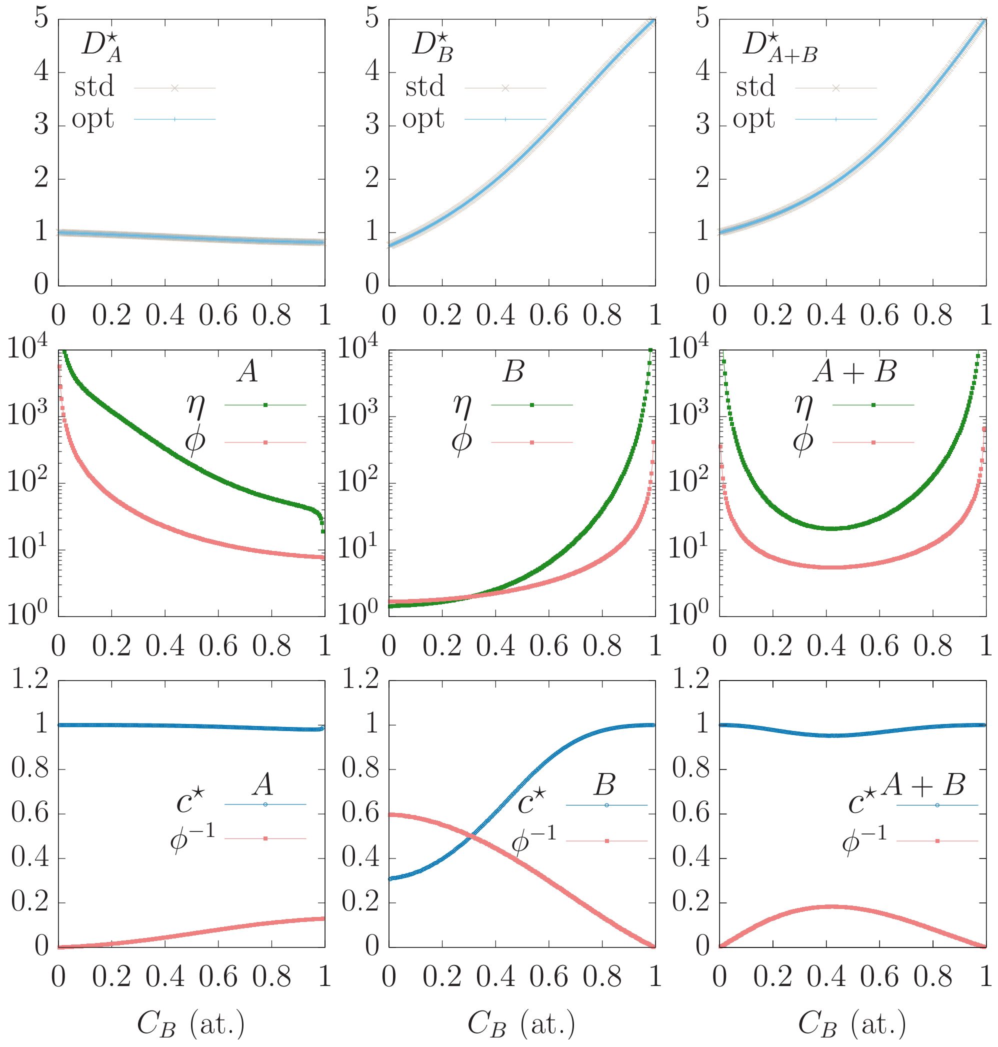


FIG. S1: Atomic diffusivities $D^\star_X$ ($X = A$, $B$ and $A+B$) for moderate dynamical trapping ($\nu_A = 1$ and $\nu_B = 5$), as a function of $C_B$, with corresponding variance reduction factor $\eta$, intra-to-extra correlation ratio $\phi$ and optimal variate $c^\star$.

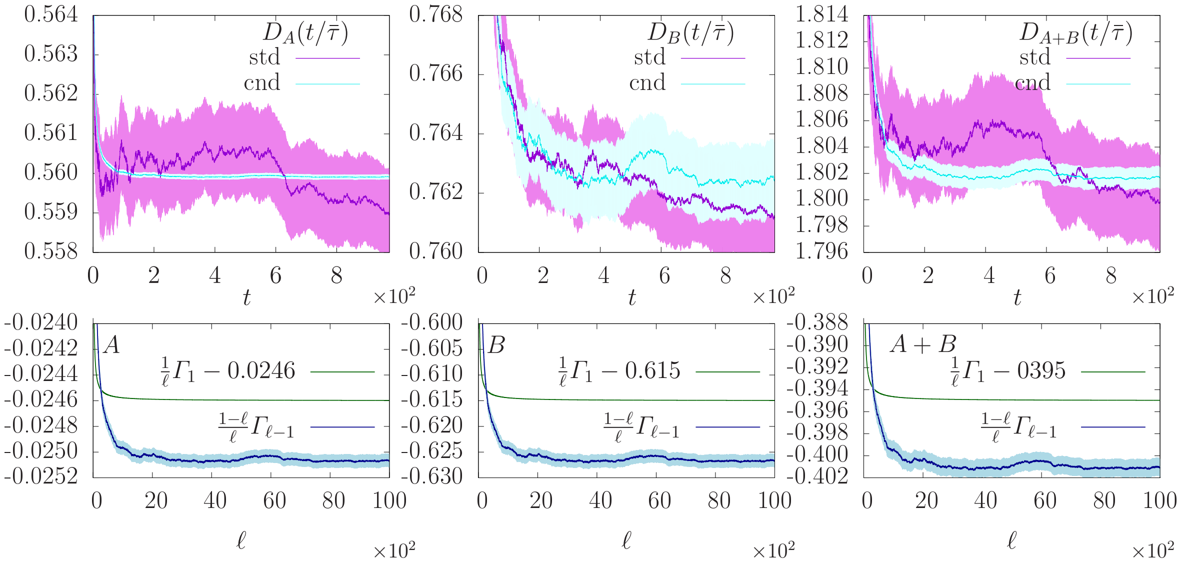


FIG. S2: Time dependence of estimated diffusion coefficients for $X$-atoms with $t = \ell\bar{\tau}$, using standard and conditioned estimators. Filled areas around the curves represent 95% confidence intervals. The confidence area around $\frac{1}{\ell}\Gamma_1$ curve is too small to be visible. Concentration of $B$ atoms is 39 at.%

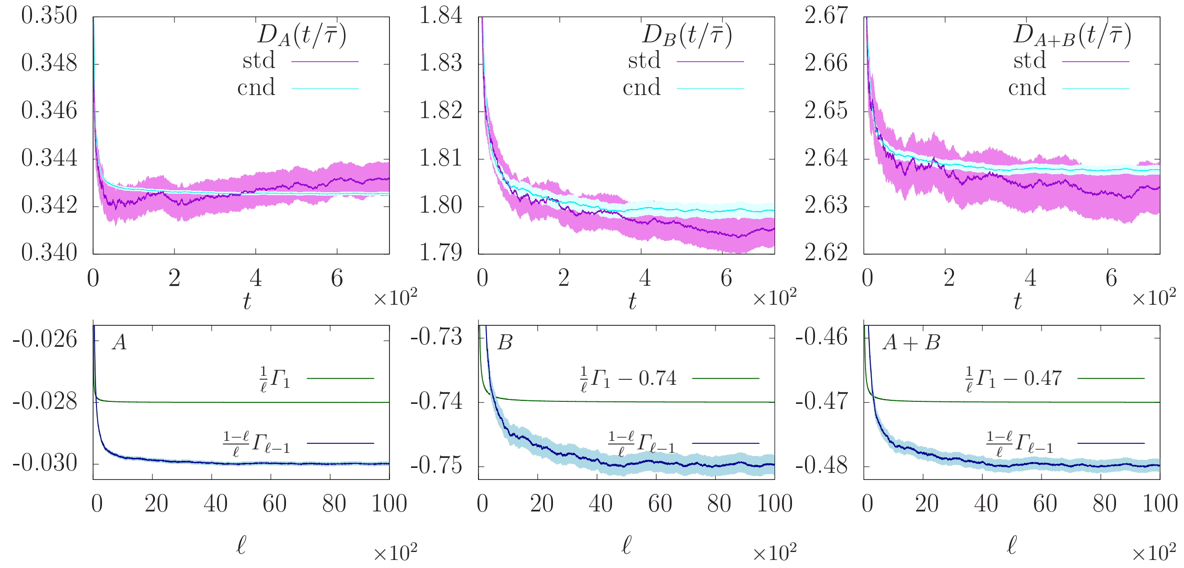


FIG. S3: Time dependence of estimated diffusion coefficients for $X$-atoms with $t = \ell\bar{\tau}$, using standard and conditioned estimators. Filled areas around the curves represent 95% confidence intervals. The confidence area around $\frac{1}{\ell}\Gamma_1$ curve is too small to be visible. Concentration of $B$ atoms is 61 at.%

## III. ALGEBRAIC DECAY OF TRANSIENT REGIME TOWARDS THE ASYMPTOTIC REGIME

The extra-correlated contributions $\Gamma_\ell$ in Fig. S2 and S3 all undergo fast algebraic decays towards their plateau values $\delta$. The $\Gamma_\ell$ curves are indeed well fitted by a law of the form $g(\ell+\ell_0)^\alpha+\delta$. Implementing the nonlinear least-squares Marquardt-Levenberg algorithm with the four fitting parameters $g$, $\ell_0$, $\alpha$ and $\delta$ yields the power-law exponents $\alpha$ for $A$, $B$ and $A+B$ diffusivities at $C_B = 39\%$: they all lie in the same 68%-confidence intervals: $-0.9835 \pm 0.0014$. We have displayed the result of the fitting procedure in Fig. S4. Note that the exponent associated with $A$-diffusivity increases as the frequency ratio is increased (see core article). The convergence features associated with mean-squared mean-displacements entails that a standard diffusive regime exhibiting short-range dependence is quickly reached as $\ell$ increases, like in the case of severe dynamical trapping studied in the core article. This property results from the

fast algebraic decay of the autocorrelation function illustrated below.

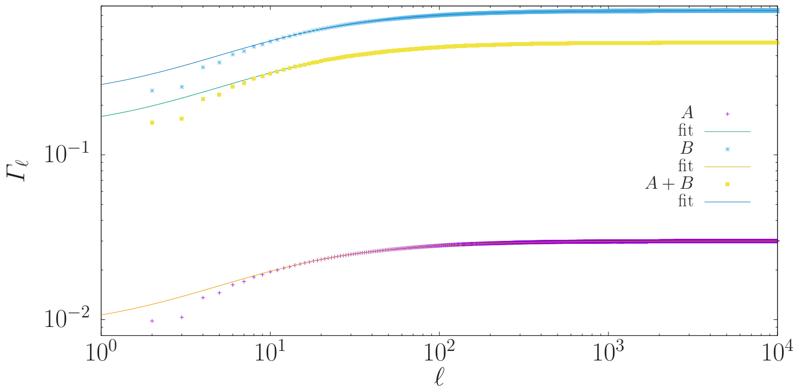


FIG. S4: Fitting of the three functions $\Gamma_\ell$ with algebraically decaying functions of the form $g(\ell+\ell_0)^\alpha+\delta$.

The autocovariance of the displacement vector given in relation (S6) defines an autocorrelation function $k \mapsto \mathbb{E}\left[\mathbf{r}_{k\to k+1}\cdot\mathbf{r}_{0\to 1}\right]$ in statistical mechanics. Its sum over the step index for $k>1$ yields the extra-correlated part. The autocorrelation function is displayed in Fig. S5 for the stoichiometric composition, a range of increasing $k$ indexes and $A+B$ diffusivity. We observe damped oscillations. The negative correlations between successive events result from the frequent occurrence of repeated exchanges of the vacancy with fast-diffusing $B$ atoms and also from the fact that the conventional kMC algorithm is rejection-free, unlike the Metropolis algorithm.

The positive and negative sub-curves both decay according to a power law of the form $h(k+k_0)^\beta$. Implementing the nonlinear least-squares Marquardt-Levenberg algorithm with the three fitting parameters $h$, $k_0$ and $\beta$ yields the power-law exponents $\beta$ lying in the intervals $-2.2197\pm0.0163$ and $-1.4849\pm0.0385$ for the upper and lower envelopes, respectively. These values being much lower than -1, the autocorrelation function undergoes a fast decay and its infinite sum over $k>1$ is bounded [S1]. This ensures that the asymptotic variance is strictly positive and bounded and thus that the diffusion process is a standard one. Diffusion is said to be anomalous when the asymptotic variance vanishes (sub-diffusion) or diverges (super-diffusion).

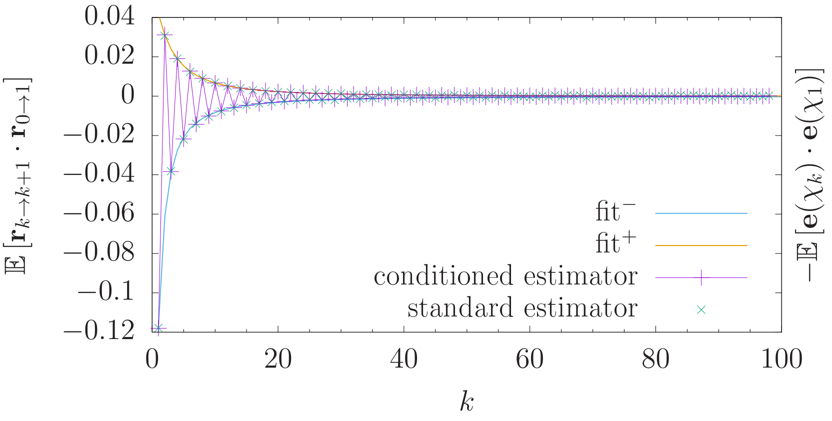


FIG. S5: Typical decay of the autocorrelation function. The standard and conditioned estimators are deduced from quantities $\mathbb{E}\left[\mathbf{r}_{k\to k+1}\cdot\mathbf{r}_{0\to 1}\right]$ and $-\mathbb{E}\left[\mathbf{e}(\chi_k)\cdot\mathbf{e}(\chi_1)\right]$, respectively, where $\mathbf{e}(\chi_k)=\mathbb{E}\left[\mathbf{r}_{k\to k+1}|\chi_k\right]$. Both estimators yield perfectly matching estimates, a result of the LTC in Eq. (S6). The curves fit$^-$ and fit$^+$ correspond to power-law fits with respect to odd and even $k$ indexes, respectively. The fitted power-law exponents are about $-1.49$ and $-2.22$, respectively. Details of the fitting procedure are given in the text. Note that the scalar product is defined by $\mathbf{x}\cdot\mathbf{y}=\mathrm{Trace}(\mathbf{x}\otimes\mathbf{y})$.

[S1] H. Rust, *Spectral analysis for stochastic processes* (2007), lecture Notes for the E2C2 / GIACS Summer School, Comorova, Romania.
